# Supplementary material for: Open Vocabulary Multi-Label Classification with Dual-Modal Decoder on Aligned Visual-Textual Features
Source: arXiv:2208.09562 source file (2023-10-07)
Supplement: Supplementary file 1 [file appendix.tex]

\section{Examples of Zero-shot Multi-label Classification by Our Approach}
We demonstrate some of the zero-shot label classification results on the NUS-WIDE dataset by our approach, as shown in Figure~\ref{fig:appendix-1} of the Appendix. Left column of each figure shows the top 8 prediction scores among various classes, which are generated from our models with ViT-L-336 backbone on $336 \times 336$ images. From them, the ones above the threshold ($0.5$ in our experiments) are chosen as the predicted labels. 
%The predicted labels for each figure are the classes corresponding to the top 8 scores, which are generated from our models with ViT-L-336 backbone on $336 \times 336$ images. 
We can see that for this challenging task, our approach can generate relevant labels in some cases. As shown quantitatively in Table 2 of the main paper text, our approach offers significant improvement over previous methods and becomes the new SOTA.

\begin{figure*}[htb]
\centering
%\vspace{-0.2cm}
%\setlength{\abovecaptionskip}{0.15cm}
%\setlength{\belowcaptionskip}{-0.25cm}
\includegraphics[width=19cm]{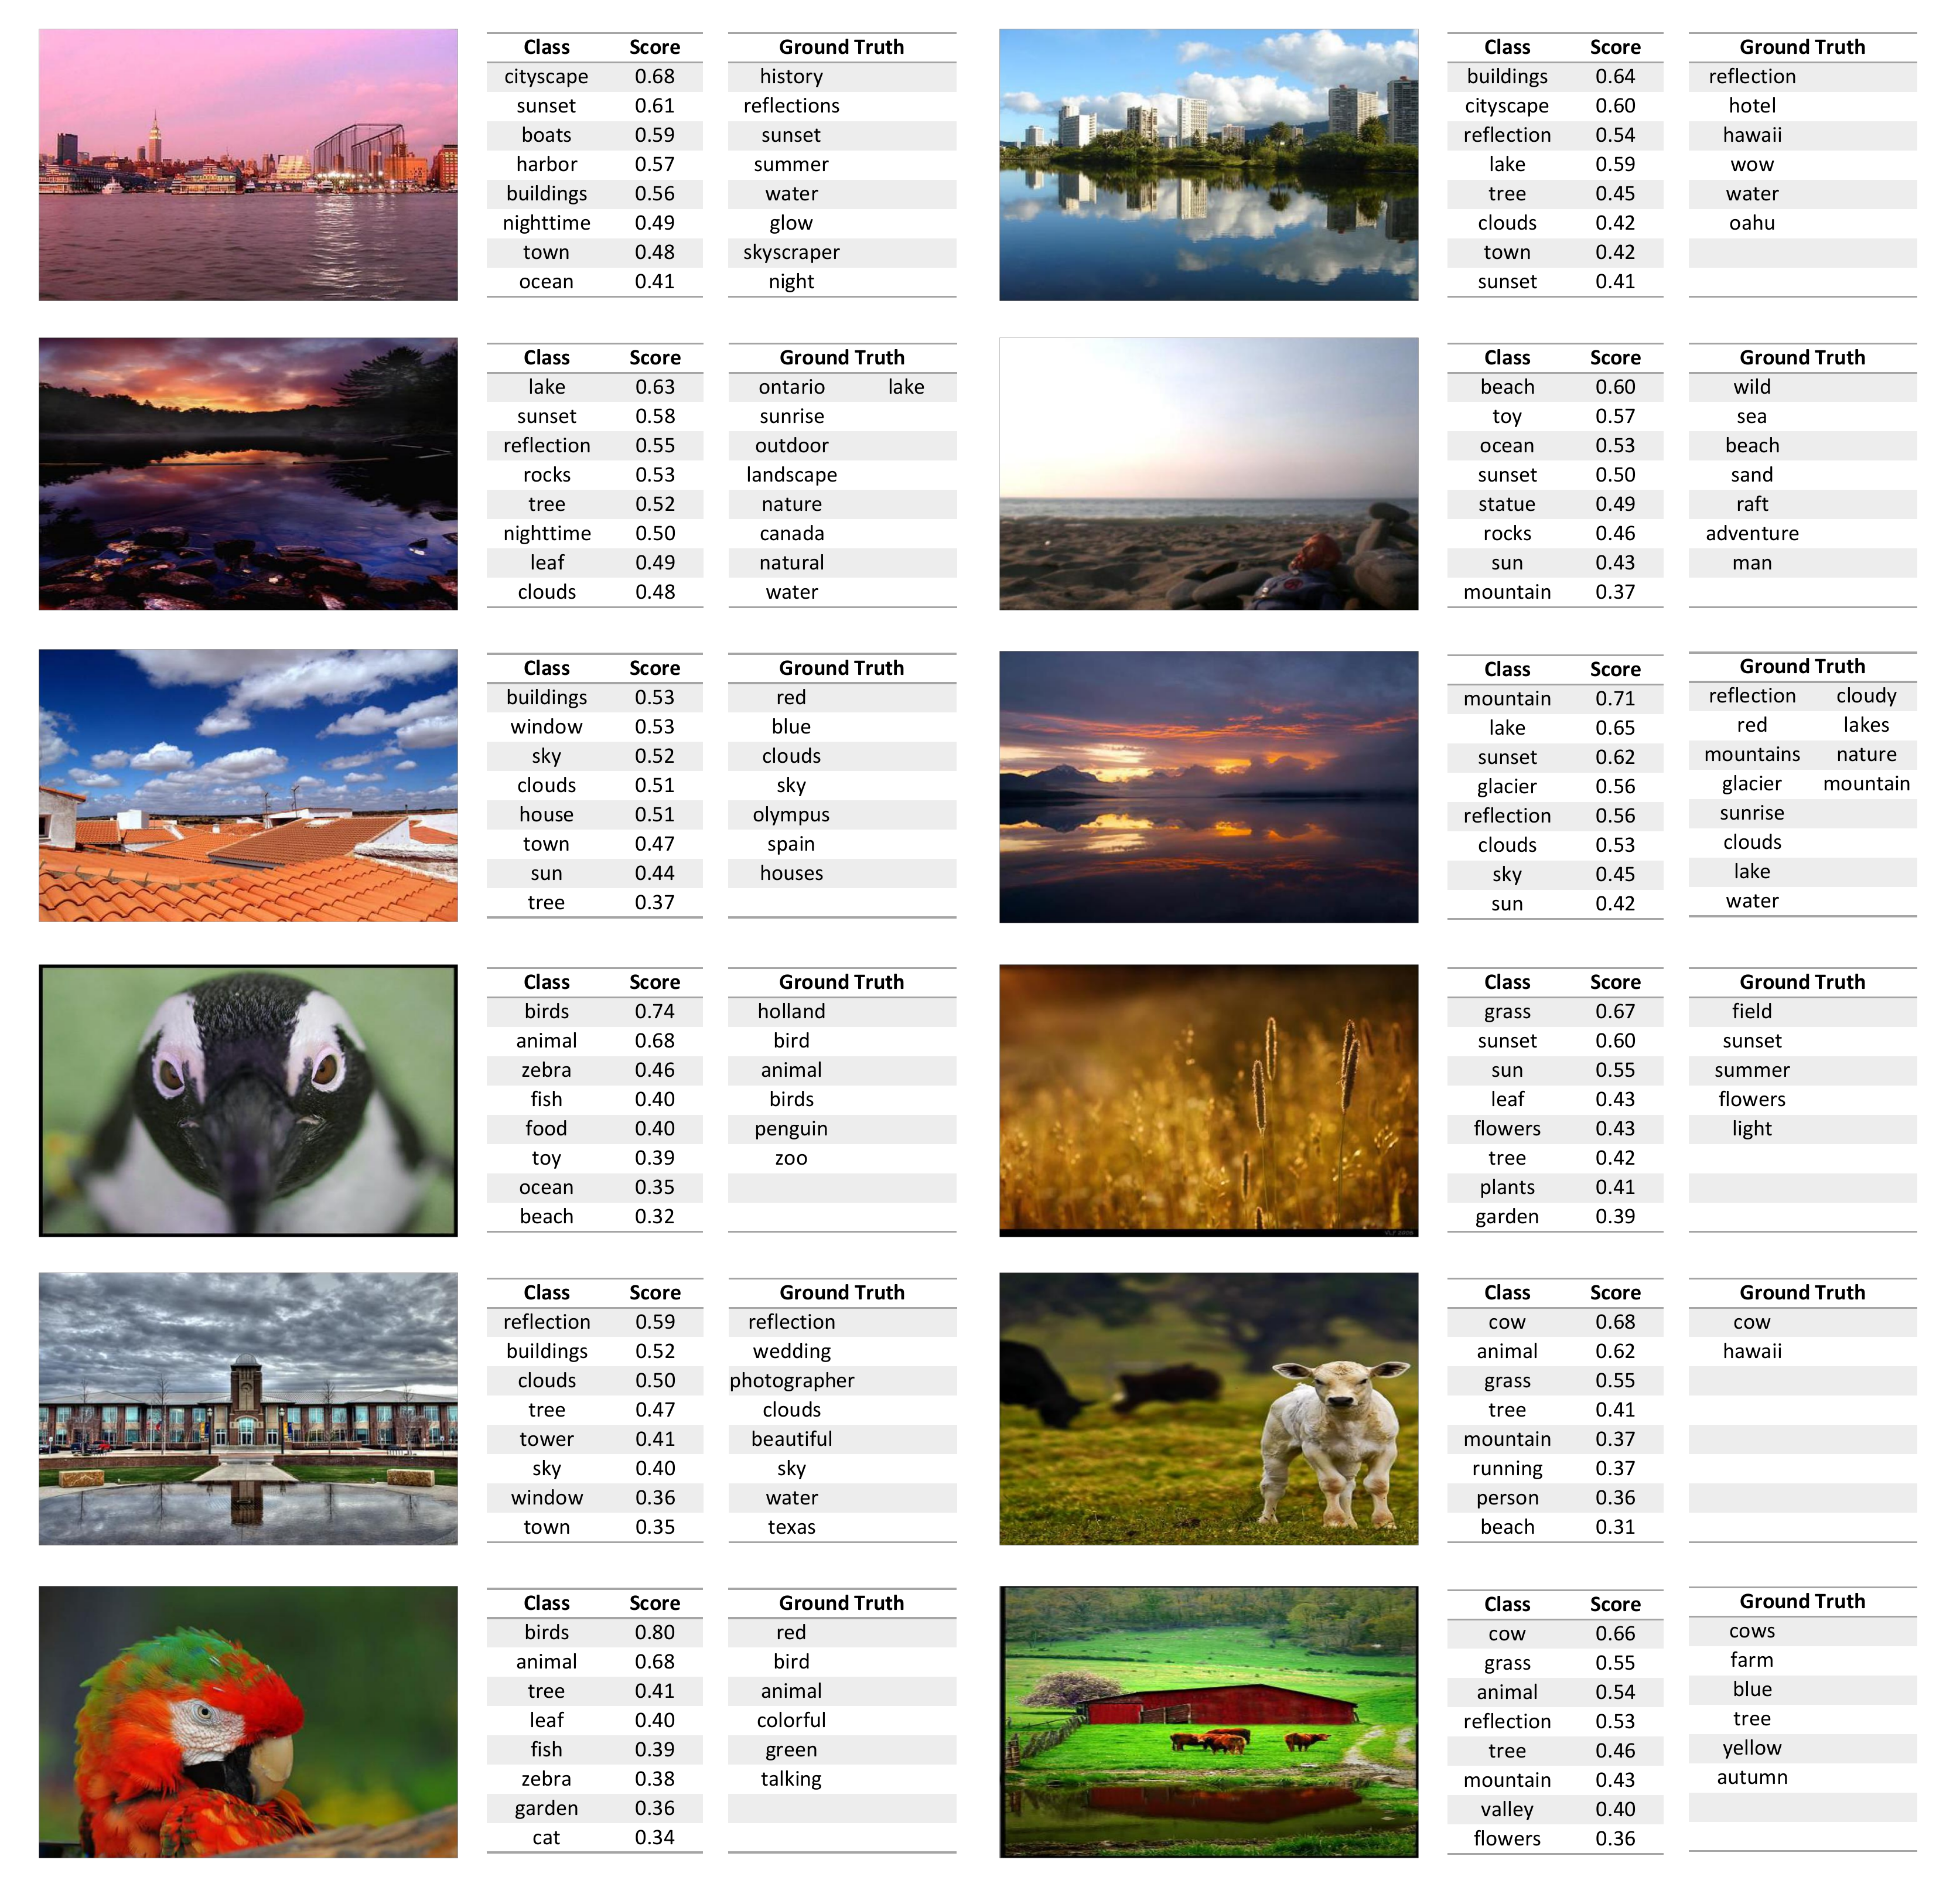}
%\vspace{-0.2cm}
\caption{Examples of zero-shot multi-label classification by our approach on the NUS-WIDE dataset.}
%\vspace{-0.2cm}
\label{fig:appendix-1}
\end{figure*}

\section{Examples of Generating Multiple Labels on Single-label Dataset}

Figure~\ref{fig:appendix-2} of the Appendix shows some examples of our approach in generating multiple labels for a single-label dataset (ImageNet-1k) after being trained on the same single-label dataset (different training and testing partitions). 
Left column of each figure shows the top 7 prediction scores among various classes, which are generated from our models with ViT-L-336 backbone on $336 \times 336$ images.
%Apart from the main sections in our paper, we also demonstrate some cases that our model trained on single-label images only can assign the single-label image with multiple labels. We make predictions on some examples from ImageNet-1k validation set,  using the model trained on ImageNet-1k(shown in Figure~\ref{fig:appendix-2}). The shown predictions are the classes corresponding to the top 7 scores, which are generated from our models with ViT-L-336 backbone on $336 \times 336$ images. 
We observe that our approach can effectively generate multiple labels that correspond to various classes/objects in the figure. This motivates us to explore the single-to-multi label classification problem in the main paper text (although in that problem, our model is tested on multiple-label datasets that were not seen during the training, and thus much more challenging).

%our model can make the predictions on the objects which exist in the image but not in the ground truth.

%\section{Source Code Release}
%We plan to release the code on GitHub later after the paper acceptance.

\begin{figure*}[htb]
\centering
%\vspace{-0.2cm}
%\setlength{\abovecaptionskip}{0.15cm}
%\setlength{\belowcaptionskip}{-0.25cm}
\includegraphics[width=19cm]{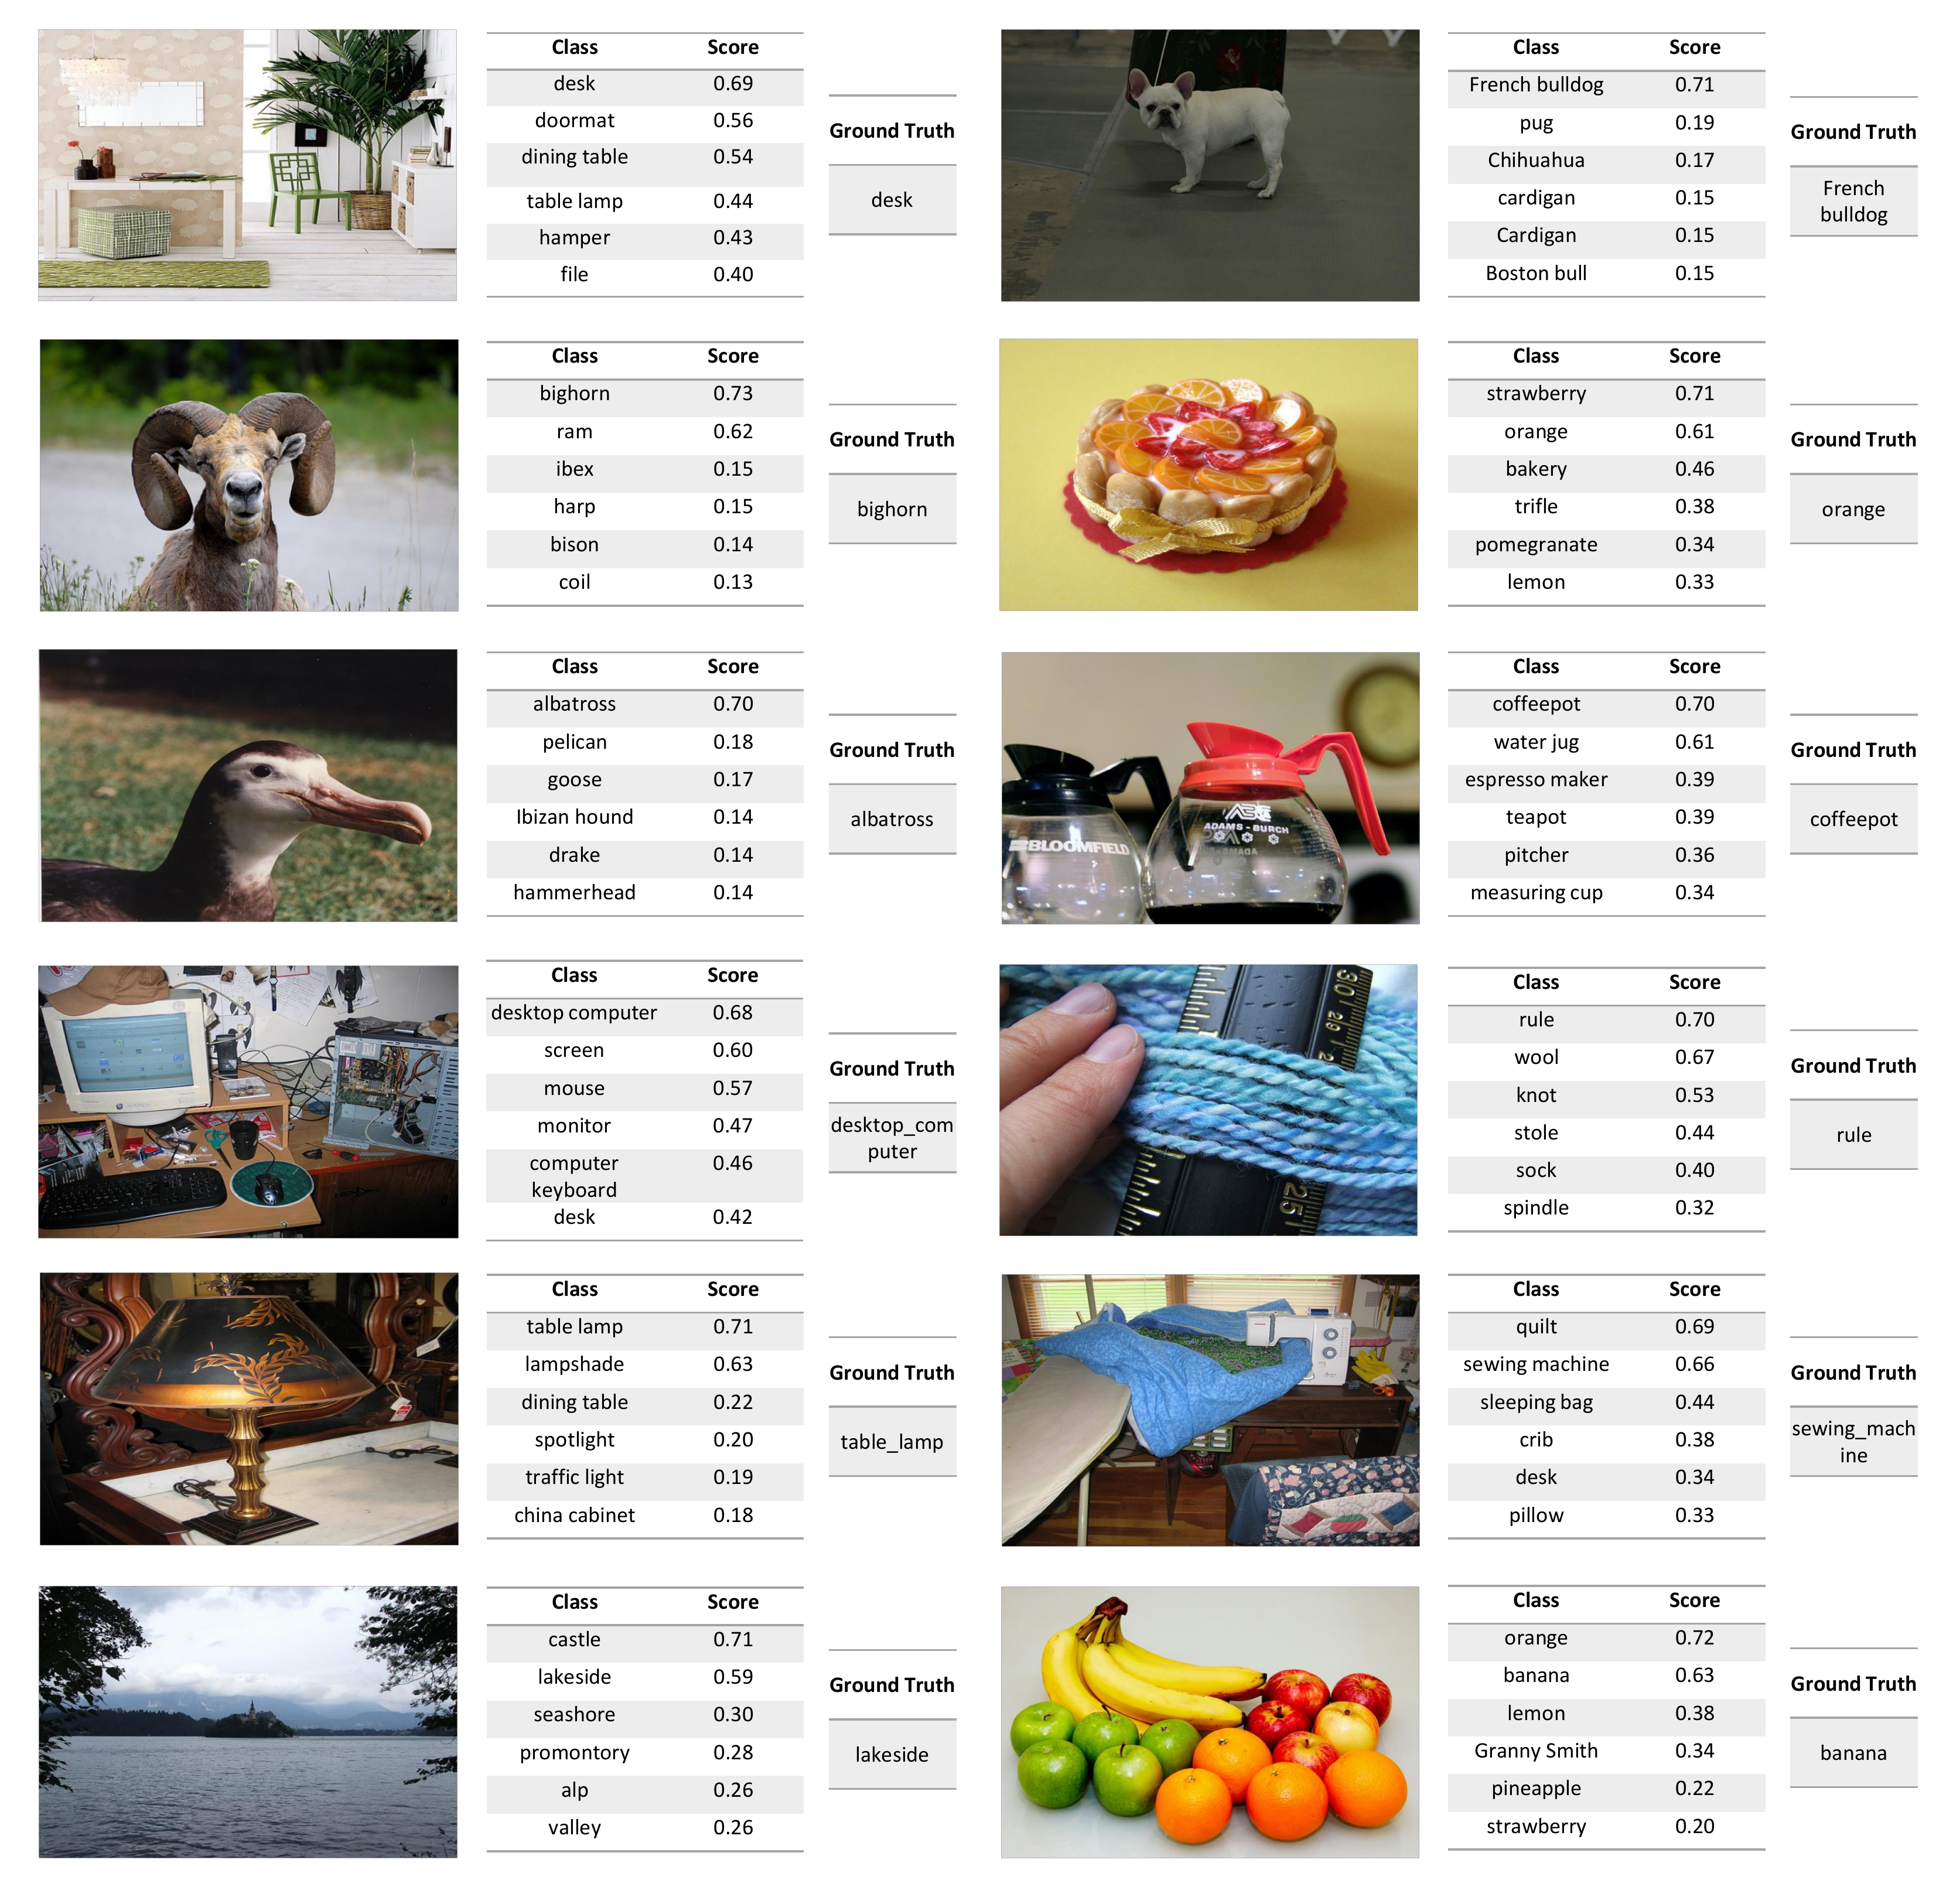}
%\vspace{-0.2cm}
\caption{Examples of our approach in generating multiple labels on a single-label dataset (ImageNet-1k) after being trained on the same single-label dataset (different training and testing partitions).}
%\vspace{-0.2cm}
\label{fig:appendix-2}
\end{figure*}
